# Supplementary material for: Rubric-based Learner Modelling via Noisy Gates Bayesian Networks for Computational Thinking Skills Assessment
Source: arXiv:2408.01221 source file (2024-08-02)
Supplement: Supplementary file 1 [file 08-appendix.tex]

\begin{table*}[htb]
\centering
\caption{Answer to the 12 schemes for a subset of pupils, expressed in terms of competencies.\label{tab:answers}}
\begin{tabular}{c|llllllllllll}
% \toprule
\textbf{Student}& \multicolumn{1}{c}{\textbf{S1}} & \multicolumn{1}{c}{\textbf{S2}} & \multicolumn{1}{c}{\textbf{S3}} & \multicolumn{1}{c}{\textbf{S4}} & \multicolumn{1}{c}{\textbf{S5}} & \multicolumn{1}{c}{\textbf{S6}} & \multicolumn{1}{c}{\textbf{S7}} & \multicolumn{1}{c}{\textbf{S8}} & \multicolumn{1}{c}{\textbf{S9}} & \multicolumn{1}{c}{\textbf{S10}}& \multicolumn{1}{c}{\textbf{S11}}& \multicolumn{1}{c}{\textbf{S12}}\\
\midrule
1   &   1D V	& 1D V	  & 1D VS	 & 1D V	     & 1D V	     & 1D V	   & 2D V	& 0D VS	& 0D V	  & 0D V	& 0D V	& 0D V \\
6   &   1D V	& 1D V	  & 1D V	 & 1D V	     & 1D V	     & 1D V	   & 0D V	& 0D V	& 0D V	  & 1D V	& 1D V	& 0D V \\
16  &   1D V	& 1D V	  & 2D V	 & 1D V	     & 1D V	     & 1D V	   & 2D V	& 2D V	& 2D V	  & 2D V	& 1D V	& 1D V \\
19  &   1D V	& 1D V	  & 2D V	 & 1D V	     & 1D V	     & 1D V	   & 2D V	& 2D V	& 2D V	  & 2D V	& 2D V	& 1D V \\
21  &   1D V	& 1D V	  & 2D V	 & 1D V	     & 1D V	     & 1D V	   & 2D V	& 2D V	& 2D V	  & 1D V	& 1D V	& 1D V \\
33  &   1D V	& 1D VS	  & 1D VS	 & 1D VSF	 & 1D VS	 & 1D VS   & 1D VS	& fail	& fail	  & fail	& fail	& fail \\
56  &   1D V	& 1D V	  & 2D V	 & 1D V	     & 1D V	     & 1D V	   & 2D V	& 2D V	& 2D V	  & 1D V	& 1D V	& 0D V \\
70  &   1D V	& 1D V	  & 1D VS	 & 1D VS	 & 1D VS	 & 1D V	   & 0D VS	& 0D VS	& 0D VS	  & 2D VS	& 2D VS	& 0D VS \\
75  &   1D V	& 1D V	  & 2D V	 & 1D V	     & 1D V	     & 1D VS   & 2D VS	& 2D VS	& 2D VS	  & 1D VS	& 1D VS	& 0D VS \\
77  &   1D VS	& 1D VS	  & 0D VS	 & 1D VS	 & 1D VS	 & 1D VSF  & 0D VS	& 0D VS	& 0D VSF  & 1D VS	& 1D VS	& 0D VS \\
79  &   1D V	& 1D V	  & 1D VS	 & 1D V	     & 1D V	     & 1D V	   & 1D VSF	& 0D VS	& 0D VS	  & 1D VS	& 1D VS	& 1D VS \\
81  &   1D V	& 1D V	  & 1D V	 & 1D VS	 & 1D V	     & 1D V	   & 2D VSF	& 0D VS	& 2D V	  & fail	& fail	& fail \\
84  &   1D V	& 1D VS	  & 1D V	 & 1D V	     & 1D V	     & 1D VS   & 1D VS	& 1D V	& 2D V	  & 2D V	& 1D V	& 1D VS \\
85  &   1D V	& 1D V	  & 1D V	 & 1D V	     & 1D V	     & 1D V	   & 0D V	& 0D V	& 0D V	  & 2D V	& 2D V	& 0D V \\
88  &   1D V	& 1D V	  & 1D V	 & 1D V	     & 1D V	     & 1D V	   & 1D VS	& 1D VS	& fail	  & fail	& fail	& fail \\
90  &   1D V	& 1D V	  & 2D V	 & 1D V	     & 1D V	     & 1D VS   & 1D VS	& 1D VS	& 2D VS	  & 1D VS	& 1D VS	& 1D VS \\
92  &   1D V	& 1D V	  & 1D V	 & 1D V	     & 1D V	     & 1D V	   & 0D V	& 0D V	& 0D VSF  & 1D VS	& 2D V	& 0D V \\
108 &   1D V	& 1D V	  & 1D V	 & 1D V	     & 1D V	     & 1D V	   & 1D V	& 2D V	& 2D V    & 1D V	& 1D V	& 0D V \\
% \bottomrule
\end{tabular}
\end{table*}

\begin{table*}[htb]
\caption{Posterior probabilities \begin{math}P(X_{rc}=1|\bm{y}^{(j)})\end{math} of all models for a subset of pupils.\label{tab:posteriors}}
\begin{center}
\begin{tabular}{c|l|ccccccccc}
  & &   \multicolumn{9}{c}{\textbf{\begin{math}P(X_{rc}=1|\bm{y}^{(j)})\end{math}}}\\ 
\textbf{Student}& \multicolumn{1}{c|}{\textbf{Model}}& { \begin{math}X_{11} \end{math}}&{ \begin{math}X_{12} \end{math}}&{ \begin{math}X_{13} \end{math}}&{ \begin{math}X_{21} \end{math}}&{ \begin{math}X_{22}\end{math}}&{\begin{math}X_{23}\end{math}}&{ \begin{math}X_{31}\end{math}}&{ \begin{math}X_{32}\end{math}}&{ \begin{math}X_{33}\end{math}}\\ 
& & {0D VSF}&{0D VS}&{0D V}&{1D VSF}&{1D VS}&{1D V}&{2D VSF}&{2D VS}&{2D V}\\ 
\midrule
\multirow{6}{*}{\textbf{1  }} & Model 1  & 0.51	&	0.60	&	0.61	&	0.54	&	0.45	&	0.98	&	0.82	&	0.30	&	0.00\\
                              & Model 1a & 1.00	&	1.00	&	1.00	&	0.90	&	0.70	&	0.36	&	0.46	&	0.02	&	0.00\\
                              & Model 1b & 1.00	&	1.00	&	1.00	&	1.00	&	1.00	&	1.00	&	0.60	&	0.21	&	0.03\\
                              & Model 2b & 1.00	&	1.00	&	1.00	&	1.00	&	1.00	&	1.00	&	0.61	&	0.22	&	0.05\\
                              & Model 3b & 1.00	&	1.00	&	1.00	&	1.00	&	1.00	&	1.00	&	0.78	&	0.57	&	0.41\\
                              & Model 4b & 1.00	&	1.00	&	1.00	&	1.00	&	1.00	&	1.00	&	0.76	&	0.51	&	0.35\\ \midrule
\multirow{6}{*}{\textbf{6  }} & Model 1  & 0.50	&	0.52	&	0.89	&	0.53	&	0.68	&	1.00	&	0.53	&	0.68	&	0.00\\
                              & Model 1a & 1.00	&	1.00	&	1.00	&	1.00	&	1.00	&	1.00	&	0.67	&	0.33	&	0.00\\
                              & Model 1b & 1.00	&	1.00	&	1.00	&	1.00	&	1.00	&	1.00	&	0.73	&	0.46	&	0.19\\
                              & Model 2b & 1.00	&	1.00	&	1.00	&	1.00	&	1.00	&	1.00	&	0.77	&	0.53	&	0.30\\
                              & Model 3b & 1.00	&	1.00	&	1.00	&	1.00	&	1.00	&	1.00	&	0.85	&	0.70	&	0.56\\
                              & Model 4b & 1.00	&	1.00	&	1.00	&	1.00	&	1.00	&	1.00	&	0.81	&	0.62	&	0.43\\ \midrule
\multirow{6}{*}{\textbf{16 }} & Model 1  & 0.50	&	0.51	&	0.61	&	0.51	&	0.55	&	0.96	&	0.58	&	0.82	&	0.99\\
                              & Model 1a & 1.00	&	1.00	&	1.00	&	1.00	&	1.00	&	1.00	&	0.90	&	0.81	&	0.71\\
                              & Model 1b & 1.00	&	1.00	&	1.00	&	1.00	&	1.00	&	1.00	&	1.00	&	1.00	&	1.00\\
                              & Model 2b & 1.00	&	1.00	&	1.00	&	1.00	&	1.00	&	1.00	&	1.00	&	1.00	&	0.99\\
                              & Model 3b & 1.00	&	1.00	&	1.00	&	1.00	&	1.00	&	1.00	&	1.00	&	1.00	&	1.00\\
                              & Model 4b & 1.00	&	1.00	&	1.00	&	1.00	&	1.00	&	1.00	&	1.00	&	1.00	&	1.00\\ \midrule
\multirow{6}{*}{\textbf{19 }} & Model 1  & 0.50	&	0.51	&	0.61	&	0.51	&	0.55	&	0.95	&	0.58	&	0.85	&	1.00\\
                              & Model 1a & 1.00	&	1.00	&	1.00	&	1.00	&	1.00	&	1.00	&	1.00	&	0.99	&	0.99\\
                              & Model 1b & 1.00	&	1.00	&	1.00	&	1.00	&	1.00	&	1.00	&	1.00	&	1.00	&	1.00\\
                              & Model 2b & 1.00	&	1.00	&	1.00	&	1.00	&	1.00	&	1.00	&	1.00	&	1.00	&	1.00\\
                              & Model 3b & 1.00	&	1.00	&	1.00	&	1.00	&	1.00	&	1.00	&	1.00	&	1.00	&	1.00\\
                              & Model 4b & 1.00	&	1.00	&	1.00	&	1.00	&	1.00	&	1.00	&	1.00	&	1.00	&	1.00\\ \midrule
\multirow{6}{*}{\textbf{21 }} & Model 1  & 0.50	&	0.51	&	0.67	&	0.51	&	0.57	&	0.96	&	0.59	&	0.83	&	0.80\\
                              & Model 1a & 1.00	&	1.00	&	1.00	&	1.00	&	1.00	&	1.00	&	0.69	&	0.38	&	0.07\\
                              & Model 1b & 1.00	&	1.00	&	1.00	&	1.00	&	1.00	&	1.00	&	0.97	&	0.95	&	0.92\\
                              & Model 2b & 1.00	&	1.00	&	1.00	&	1.00	&	1.00	&	1.00	&	0.99	&	0.97	&	0.96\\
                              & Model 3b & 1.00	&	1.00	&	1.00	&	1.00	&	1.00	&	1.00	&	1.00	&	1.00	&	1.00\\
                              & Model 4b & 1.00	&	1.00	&	1.00	&	1.00	&	1.00	&	1.00	&	1.00	&	1.00	&	1.00\\ \midrule
\multirow{6}{*}{\textbf{33 }} & Model 1  & 0.00	&	0.00	&	0.00	&	0.00	&	1.00	&	0.00	&	0.00	&	0.00	&	0.00\\
                              & Model 1a & 0.00	&	0.00	&	0.00	&	0.00	&	0.00	&	0.00	&	0.00	&	0.00	&	0.00\\
                              & Model 1b & 1.00	&	1.00	&	0.52	&	1.00	&	1.00	&	0.05	&	0.59	&	0.30	&	0.00\\
                              & Model 2b & 1.00	&	1.00	&	0.53	&	1.00	&	1.00	&	0.08	&	0.58	&	0.30	&	0.00\\
                              & Model 3b & 1.00	&	1.00	&	0.69	&	1.00	&	1.00	&	0.39	&	0.63	&	0.33	&	0.03\\
                              & Model 4b & 1.00	&	1.00	&	0.72	&	1.00	&	1.00	&	0.46	&	0.63	&	0.33	&	0.05\\ \midrule
\multirow{6}{*}{\textbf{56 }} & Model 1  & 0.50	&	0.51	&	0.79	&	0.52	&	0.60	&	0.90	&	0.63	&	0.91	&	0.45\\
                              & Model 1a & 1.00	&	1.00	&	1.00	&	1.00	&	1.00	&	1.00	&	0.67	&	0.34	&	0.01\\
                              & Model 1b & 1.00	&	1.00	&	1.00	&	1.00	&	1.00	&	1.00	&	0.98	&	0.96	&	0.94\\
                              & Model 2b & 1.00	&	1.00	&	1.00	&	1.00	&	1.00	&	1.00	&	0.99	&	0.97	&	0.96\\
                              & Model 3b & 1.00	&	1.00	&	1.00	&	1.00	&	1.00	&	1.00	&	1.00	&	1.00	&	1.00\\
                              & Model 4b & 1.00	&	1.00	&	1.00	&	1.00	&	1.00	&	1.00	&	1.00	&	1.00	&	1.00\\ \midrule
\multirow{6}{*}{\textbf{70 }} & Model 1  & 0.51	&	0.69	&	0.66	&	0.57	&	1.00	&	0.00	&	0.99	&	0.00	&	0.00\\
                              & Model 1a & 1.00	&	1.00	&	0.00	&	0.84	&	0.53	&	0.00	&	0.42	&	0.00	&	0.00\\
                              & Model 1b & 1.00	&	1.00	&	0.11	&	1.00	&	0.99	&	0.09	&	0.85	&	0.69	&	0.00\\
                              & Model 2b & 1.00	&	1.00	&	0.61	&	1.00	&	1.00	&	0.57	&	0.86	&	0.71	&	0.00\\
                              & Model 3b & 1.00	&	1.00	&	0.93	&	1.00	&	1.00	&	0.91	&	0.94	&	0.88	&	0.12\\
                              & Model 4b & 1.00	&	1.00	&	0.87	&	1.00	&	1.00	&	0.86	&	0.94	&	0.89	&	0.15\\
\end{tabular}
\end{center}
\end{table*}

\begin{table*}[htb]
\ContinuedFloat
\caption{Posterior probabilities \begin{math}P(X_{rc}=1|\bm{y}^{(j)})\end{math} of all models for a subset of pupils (continued).}
\begin{center}
\begin{tabular}{c|l|ccccccccc}
  & &   \multicolumn{9}{c}{\textbf{\begin{math}P(X_{rc}=1|\bm{y}^{(j)})\end{math}}}\\ 
\textbf{Student}& \multicolumn{1}{c|}{\textbf{Model}}& { \begin{math}X_{11} \end{math}}&{ \begin{math}X_{12} \end{math}}&{ \begin{math}X_{13} \end{math}}&{ \begin{math}X_{21} \end{math}}&{ \begin{math}X_{22}\end{math}}&{\begin{math}X_{23}\end{math}}&{ \begin{math}X_{31}\end{math}}&{ \begin{math}X_{32}\end{math}}&{ \begin{math}X_{33}\end{math}}\\ 
& & {0D VSF}&{0D VS}&{0D V}&{1D VSF}&{1D VS}&{1D V}&{2D VSF}&{2D VS}&{2D V}\\ 
\midrule
\multirow{6}{*}{\textbf{75 }} & Model 1  & 0.51	&	0.56	&	0.36	&	0.54	&	0.29	&	0.99	&	0.71	&	0.95	&	0.00\\
                              & Model 1a & 1.00	&	1.00	&	0.38	&	1.00	&	0.99	&	0.26	&	0.70	&	0.40	&	0.00\\
                              & Model 1b & 1.00	&	1.00	&	0.99	&	1.00	&	1.00	&	0.98	&	0.97	&	0.95	&	0.01\\
                              & Model 2b & 1.00	&	1.00	&	1.00	&	1.00	&	1.00	&	1.00	&	0.99	&	0.98	&	0.03\\
                              & Model 3b & 1.00	&	1.00	&	1.00	&	1.00	&	1.00	&	1.00	&	1.00	&	0.99	&	0.65\\
                              & Model 4b & 1.00	&	1.00	&	1.00	&	1.00	&	1.00	&	1.00	&	1.00	&	0.99	&	0.68\\ \midrule
\multirow{6}{*}{\textbf{77 }} & Model 1  & 0.61	&	0.66	&	0.00	&	0.48	&	0.98	&	0.00	&	0.02	&	0.00	&	0.00\\
                              & Model 1a & 1.00	&	1.00	&	0.00	&	0.95	&	0.85	&	0.00	&	0.04	&	0.00	&	0.00\\
                              & Model 1b & 1.00	&	1.00	&	0.02	&	1.00	&	1.00	&	0.00	&	0.49	&	0.14	&	0.00\\
                              & Model 2b & 1.00	&	1.00	&	0.07	&	1.00	&	1.00	&	0.00	&	0.55	&	0.21	&	0.00\\
                              & Model 3b & 1.00	&	1.00	&	0.17	&	1.00	&	1.00	&	0.00	&	0.61	&	0.30	&	0.00\\
                              & Model 4b & 1.00	&	1.00	&	0.13	&	1.00	&	1.00	&	0.00	&	0.58	&	0.24	&	0.00\\ \midrule
\multirow{6}{*}{\textbf{79 }} & Model 1  & 0.51	&	0.65	&	0.81	&	0.77	&	0.80	&	0.23	&	0.29	&	0.00	&	0.00\\
                              & Model 1a & 1.00	&	1.00	&	0.04	&	1.00	&	0.98	&	0.00	&	0.17	&	0.00	&	0.00\\
                              & Model 1b & 1.00	&	1.00	&	0.97	&	1.00	&	1.00	&	0.97	&	0.59	&	0.25	&	0.06\\
                              & Model 2b & 1.00	&	1.00	&	1.00	&	1.00	&	1.00	&	1.00	&	0.64	&	0.32	&	0.11\\
                              & Model 3b & 1.00	&	1.00	&	1.00	&	1.00	&	1.00	&	1.00	&	0.70	&	0.42	&	0.20\\
                              & Model 4b & 1.00	&	1.00	&	1.00	&	1.00	&	1.00	&	1.00	&	0.65	&	0.33	&	0.13\\ \midrule
\multirow{6}{*}{\textbf{81 }} & Model 1  & 0.03	&	0.00	&	0.00	&	0.00	&	0.00	&	1.00	&	0.00	&	0.00	&	0.00\\
                              & Model 1a & 0.01	&	0.00	&	0.00	&	0.00	&	0.00	&	0.00	&	0.00	&	0.00	&	0.00\\
                              & Model 1b & 1.00	&	1.00	&	1.00	&	1.00	&	1.00	&	1.00	&	0.91	&	0.21	&	0.03\\
                              & Model 2b & 1.00	&	1.00	&	1.00	&	1.00	&	1.00	&	1.00	&	0.91	&	0.26	&	0.02\\
                              & Model 3b & 1.00	&	1.00	&	1.00	&	1.00	&	1.00	&	1.00	&	0.95	&	0.67	&	0.44\\
                              & Model 4b & 1.00	&	1.00	&	1.00	&	1.00	&	1.00	&	1.00	&	0.96	&	0.70	&	0.50\\ \midrule
\multirow{6}{*}{\textbf{84 }} & Model 1  & 0.50	&	0.53	&	0.82	&	0.53	&	0.81	&	1.00	&	0.85	&	0.37	&	0.00\\
                              & Model 1a & 1.00	&	1.00	&	1.00	&	1.00	&	1.00	&	1.00	&	0.50	&	0.00	&	0.00\\
                              & Model 1b & 1.00	&	1.00	&	1.00	&	1.00	&	1.00	&	1.00	&	0.51	&	0.01	&	0.00\\
                              & Model 2b & 1.00	&	1.00	&	1.00	&	1.00	&	1.00	&	1.00	&	0.52	&	0.05	&	0.01\\
                              & Model 3b & 1.00	&	1.00	&	1.00	&	1.00	&	1.00	&	1.00	&	0.74	&	0.48	&	0.41\\
                              & Model 4b & 1.00	&	1.00	&	1.00	&	1.00	&	1.00	&	1.00	&	0.82	&	0.64	&	0.57\\ \midrule
\multirow{6}{*}{\textbf{85 }} & Model 1  & 0.50	&	0.52	&	0.89	&	0.52	&	0.59	&	1.00	&	0.60	&	1.00	&	0.00\\
                              & Model 1a & 1.00	&	1.00	&	1.00	&	1.00	&	1.00	&	1.00	&	0.67	&	0.33	&	0.00\\
                              & Model 1b & 1.00	&	1.00	&	1.00	&	1.00	&	1.00	&	1.00	&	0.74	&	0.48	&	0.21\\
                              & Model 2b & 1.00	&	1.00	&	1.00	&	1.00	&	1.00	&	1.00	&	0.71	&	0.42	&	0.13\\
                              & Model 3b & 1.00	&	1.00	&	1.00	&	1.00	&	1.00	&	1.00	&	0.95	&	0.90	&	0.85\\
                              & Model 4b & 1.00	&	1.00	&	1.00	&	1.00	&	1.00	&	1.00	&	0.95	&	0.91	&	0.86\\ \midrule
\multirow{6}{*}{\textbf{88 }} & Model 1  & 0.01	&	0.00	&	0.00	&	0.00	&	0.00	&	1.00	&	0.00	&	0.00	&	0.00\\
                              & Model 1a & 0.00	&	0.00	&	0.00	&	0.00	&	0.00	&	0.00	&	0.00	&	0.00	&	0.00\\
                              & Model 1b & 1.00	&	1.00	&	1.00	&	1.00	&	1.00	&	1.00	&	0.70	&	0.40	&	0.19\\
                              & Model 2b & 1.00	&	1.00	&	1.00	&	1.00	&	1.00	&	1.00	&	0.72	&	0.44	&	0.21\\
                              & Model 3b & 1.00	&	1.00	&	1.00	&	1.00	&	1.00	&	1.00	&	0.79	&	0.58	&	0.37\\
                              & Model 4b & 1.00	&	1.00	&	1.00	&	1.00	&	1.00	&	1.00	&	0.77	&	0.53	&	0.30\\ \midrule
\multirow{6}{*}{\textbf{90 }} & Model 1  & 0.50	&	0.55	&	0.74	&	0.53	&	0.92	&	0.99	&	0.98	&	0.02	&	0.00\\
                              & Model 1a & 1.00	&	1.00	&	0.64	&	1.00	&	1.00	&	0.28	&	0.50	&	0.00	&	0.00\\
                              & Model 1b & 1.00	&	1.00	&	0.97	&	1.00	&	1.00	&	0.95	&	0.51	&	0.03	&	0.00\\
                              & Model 2b & 1.00	&	1.00	&	1.00	&	1.00	&	1.00	&	1.00	&	0.64	&	0.28	&	0.00\\
                              & Model 3b & 1.00	&	1.00	&	1.00	&	1.00	&	1.00	&	1.00	&	0.84	&	0.69	&	0.30\\
                              & Model 4b & 1.00	&	1.00	&	1.00	&	1.00	&	1.00	&	1.00	&	0.84	&	0.67	&	0.30\\ \midrule
\multirow{6}{*}{\textbf{92 }} & Model 1  & 0.55	&	0.40	&	0.41	&	0.33	&	0.13	&	1.00	&	0.46	&	0.05	&	0.00\\
                              & Model 1a & 1.00	&	0.99	&	0.99	&	0.76	&	0.70	&	0.68	&	0.13	&	0.00	&	0.00\\
                              & Model 1b & 1.00	&	1.00	&	1.00	&	1.00	&	1.00	&	1.00	&	0.59	&	0.19	&	0.01\\
                              & Model 2b & 1.00	&	1.00	&	1.00	&	1.00	&	1.00	&	1.00	&	0.63	&	0.27	&	0.01\\
                              & Model 3b & 1.00	&	1.00	&	1.00	&	1.00	&	1.00	&	1.00	&	0.79	&	0.58	&	0.41\\
                              & Model 4b & 1.00	&	1.00	&	1.00	&	1.00	&	1.00	&	1.00	&	0.78	&	0.57	&	0.41\\ \midrule
\multirow{6}{*}{\textbf{108}} & Model 1  & 0.50	&	0.51	&	0.89	&	0.52	&	0.62	&	1.00	&	0.61	&	1.00	&	0.00\\
                              & Model 1a & 1.00	&	1.00	&	1.00	&	1.00	&	1.00	&	1.00	&	0.67	&	0.33	&	0.00\\
                              & Model 1b & 1.00	&	1.00	&	1.00	&	1.00	&	1.00	&	1.00	&	0.67	&	0.35	&	0.02\\
                              & Model 2b & 1.00	&	1.00	&	1.00	&	1.00	&	1.00	&	1.00	&	0.69	&	0.38	&	0.07\\
                              & Model 3b & 1.00	&	1.00	&	1.00	&	1.00	&	1.00	&	1.00	&	0.95	&	0.91	&	0.86\\
                              & Model 4b & 1.00	&	1.00	&	1.00	&	1.00	&	1.00	&	1.00	&	0.95	&	0.91	&	0.86\\
% \bottomrule
\end{tabular}
\end{center}
\end{table*}
